# Supplementary material for: R2E-Gym: Procedural Environments and Hybrid Verifiers for Scaling Open-Weights SWE Agents
Source: arXiv:2504.07164 source file (2025-04-09)
Supplement: Supplementary file 1 [file X_supp.tex]

\newpage

\section{Inference Time Scaling}
\input{tables/verif-ablation}
